# Supplementary material for: An Empirical Study of the Generalization Ability of Lidar 3D Object Detectors to Unseen Domains
Source: arXiv:2402.17562 source file (2024-02-27)
Supplement: Supplementary file 1 [file table_weather_voxel_size.tex]

\begin{table*}[h!]
\centering

\setlength{\tabcolsep}{2pt}
\resizebox{\linewidth}{!}{
\begin{tabular}{ccccccccccccc}
\toprule
& \multicolumn{6}{c|}{Source Domain - Waymo} & \multicolumn{6}{c}{Target Domain - Kirk} \\ \hline
\multicolumn{1}{c|}{} & \multicolumn{3}{c|}{Veh. 3D-AP}& \multicolumn{3}{c|}{Ped. 3D-AP}& \multicolumn{3}{c|}{Veh. 3D-AP}& \multicolumn{3}{c}{Ped. 3D-AP}\\
\multicolumn{1}{c|}{\multirow{-2}{*}{Voxel Size}} & LEVEL\_1& LEVEL\_2& \multicolumn{1}{c|}{mAP} & LEVEL\_1& LEVEL\_2& \multicolumn{1}{c|}{mAP} & LEVEL\_1& LEVEL\_2& \multicolumn{1}{c|}{mAP} & LEVEL\_1& LEVEL\_2& mAP \\ \hline
\multicolumn{1}{c|}{(0.1, 0.1, 0.1)}& {\color[HTML]{FF0000} \textbf{75.53}} & {\color[HTML]{FF0000} \textbf{67.00}} & \multicolumn{1}{c|}{{\color[HTML]{FF0000} \textbf{71.27}}} & {\color[HTML]{FF0000} \textbf{72.71}} & \second{63.71}& \multicolumn{1}{c|}{\second{68.21}}& {\color[HTML]{FF0000} \textbf{60.60}} & {\color[HTML]{FF0000} \textbf{50.96}} & \multicolumn{1}{c|}{{\color[HTML]{FF0000} \textbf{55.78}}} & \second{27.90}& \second{19.56}& \second{23.73}\\
\multicolumn{1}{c|}{(0.1, 0.1, 0.15)} & \second{75.26}& \second{66.75}& \multicolumn{1}{c|}{\second{71.01}}& {\color[HTML]{FF0000} \textbf{72.71}} & {\color[HTML]{FF0000} \textbf{63.74}} & \multicolumn{1}{c|}{{\color[HTML]{FF0000} \textbf{68.23}}} & \second{59.77}& \second{50.26}& \multicolumn{1}{c|}{\second{55.02}}& {\color[HTML]{FF0000} \textbf{28.04}} & {\color[HTML]{FF0000} \textbf{19.65}} & {\color[HTML]{FF0000} \textbf{23.85}} \\
\multicolumn{1}{c|}{(0.15, 0.1, 0.15)}& 75.22 & \second{66.75}& \multicolumn{1}{c|}{70.99} & 70.89 & 61.93 & \multicolumn{1}{c|}{66.41} & 59.71 & 50.10 & \multicolumn{1}{c|}{54.91} & 25.79 & 18.12 & 21.96 \\
\multicolumn{1}{c|}{(0.1, 0.1, 0.175)}& 74.51 & 65.99 & \multicolumn{1}{c|}{70.25} & 71.79 & 62.80 & \multicolumn{1}{c|}{67.30} & 58.96 & 49.52 & \multicolumn{1}{c|}{54.24} & 25.07 & 17.60 & 21.34 \\
\multicolumn{1}{c|}{(0.1, 0.1, 0.2)}& 73.18 & 64.62 & \multicolumn{1}{c|}{68.90} & 69.08 & 59.99 & \multicolumn{1}{c|}{64.54} & 56.93 & 47.50 & \multicolumn{1}{c|}{52.22} & 21.85 & 15.34 & 18.60 \\ \hline
\end{tabular}}
\caption{Voxel encoding of PVRCNN in Waymo datasets. The best results are indicated in red and the second-best results are indicated in blue.}
\label{weather_voxel_encoding}
\vspace{-1em}
\end{table*}
