# Supplementary material for: An Empirical Study of the Generalization Ability of Lidar 3D Object Detectors to Unseen Domains
Source: arXiv:2402.17562 source file (2024-02-27)
Supplement: Supplementary file 2 [file gt_sampling_tp_fp.tex]

\begin{figure*}[t!]
	\centering
	\includegraphics[scale=.15]{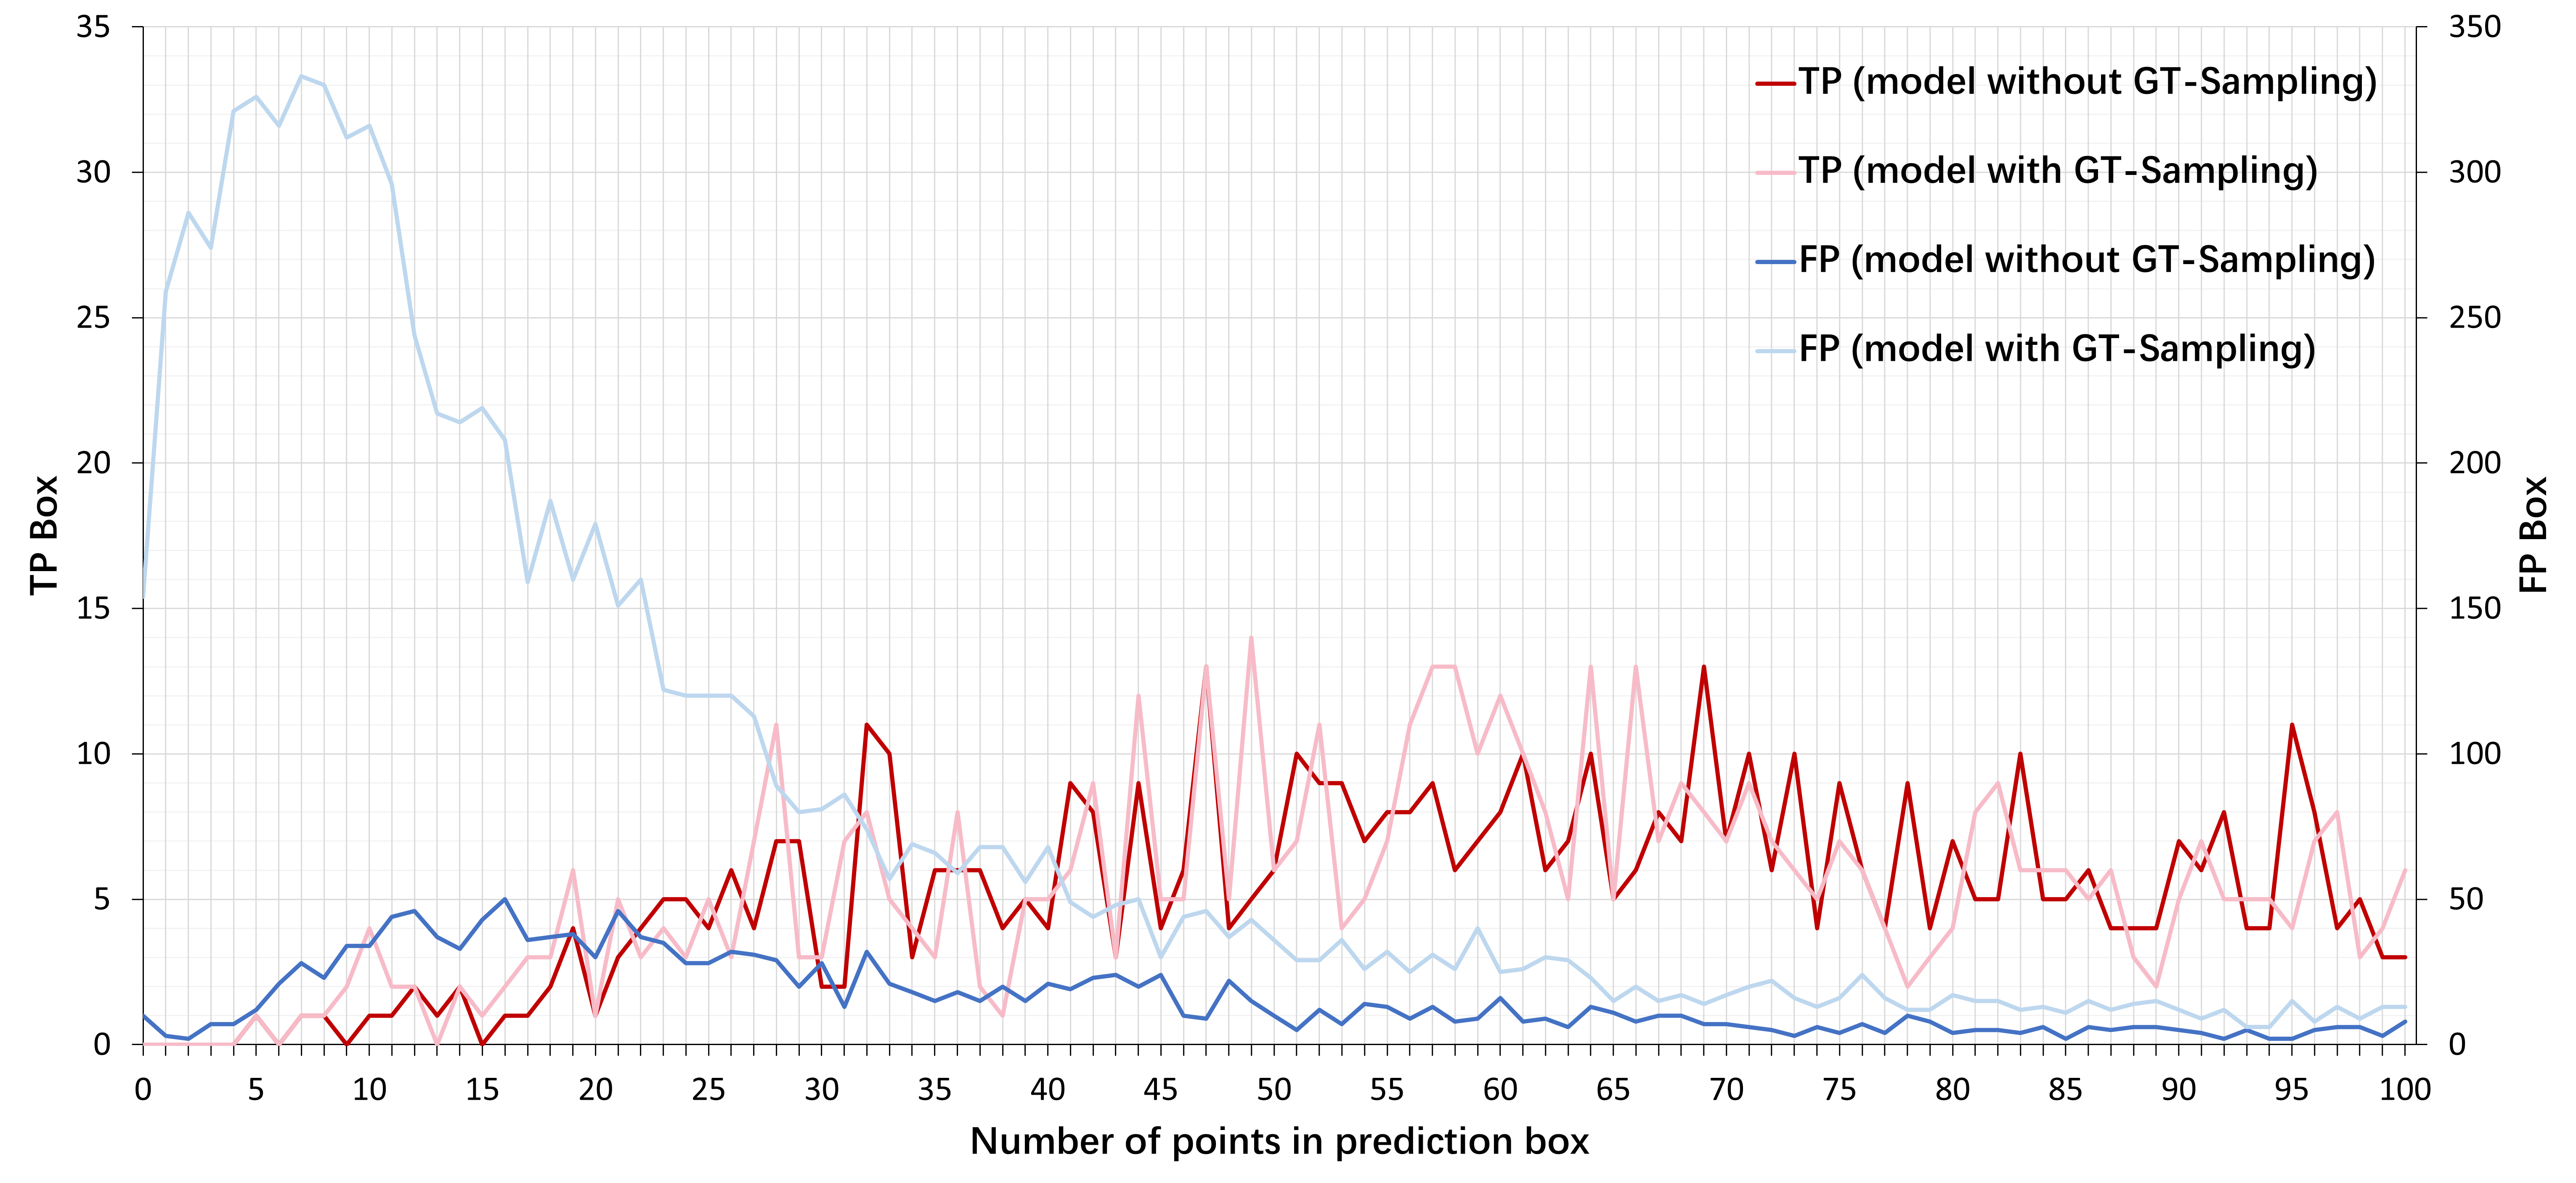}
	\caption{Number of True Positives and False Positives predicted by PVRCNN for the pedestrian class on KITTI-64 $\rightarrow$ KITTI-16.} 
	\label{gtsampling_tp_fp}
\end{figure*}
