# Supplementary material for: An Empirical Study of the Generalization Ability of Lidar 3D Object Detectors to Unseen Domains
Source: arXiv:2402.17562 source file (2024-02-27)
Supplement: Supplementary file 3 [file models_location.tex]

\begin{figure*}[ht!]
     \centering
     \begin{subfigure}[b]{0.27\textwidth}
         \centering
         \includegraphics[width=\textwidth]{iccv2023AuthorKit/Appendix_Figures/supp_scatter1.pdf}
         \caption{Waymo $\rightarrow$ KITTI}
         \label{subfig:WTK}
     \end{subfigure}
     \hfill
     \begin{subfigure}[b]{0.32\textwidth}
         \centering
         \includegraphics[width=\textwidth]{iccv2023AuthorKit/Appendix_Figures/supp_scatter3.pdf}
         \caption{Waymo $\rightarrow$ nuScenes}
         \label{subfig:WTN}
     \end{subfigure}
     \hfill
     \begin{subfigure}[b]{0.27\textwidth}
         \centering
         \includegraphics[width=\textwidth]{iccv2023AuthorKit/Appendix_Figures/supp_scatter2.pdf}
         \caption{nuScenes $\rightarrow$ KITTI}
         \label{subfig:NTK}
     \end{subfigure}
        \caption{An overview of different arcitecture OOD performance across various geographical locations.}
        \label{fig:three graphs}
\end{figure*}
