# Supplementary material for: An Empirical Study of the Generalization Ability of Lidar 3D Object Detectors to Unseen Domains
Source: arXiv:2402.17562 source file (2024-02-27)
Supplement: Supplementary file 4 [file multiclass_kitti.tex]

\begin{table*}[!t]
    \centering
    \adjustbox{width=\linewidth}{\begin{tabular}{c|c|ccc|ccc}
    \hline
        \multirow{2}{*}{Models} & \multirow{2}{*}{Anchors} & \multicolumn{3}{c|}{Waymo} & \multicolumn{3}{c}{Waymo $\rightarrow$ KITTI} \\ 
        ~ & ~ & Vehicle  & Pedestrian & Cyclist & Vehicle  & Pedestrian & Cyclist \\ \hline
        \multirow{2}{*}{Multi-class Training} & Training & 62.77/54.65 & 49.4/41.88 & 53.77/51.73 & 47.80 / 7.88 & 48.23 / 44.82 & 49.50 / 44.77 \\ 
        ~ & Best performing & N/A & N/A & N/A & 79.74 / 64.36 & 51.48 / 49.31 & 60.15 / 55.97 \\ 
        \midrule
        \multirow{2}{*}{Single Class Training} & Training & 66.68/58.31 & 51.42/43.68 & 57.01/54.92 & 52.42 / 12.62 & 45.20 / 42.31 & 50.94 / 44.48 \\ 
        ~ & Best performing & N/A & N/A & N/A & 80.23 / 66.72 & 49.16 / 46.10 & 60.43 / 55.69 \\ \hline
    \end{tabular}}
    \caption{Multiclass vs Singleclass training on Waymo $\rightarrow$ KITTI.}
    \label{tab:multiclass_kitti}
\end{table*}
