# Supplementary material for: An Empirical Study of the Generalization Ability of Lidar 3D Object Detectors to Unseen Domains
Source: arXiv:2402.17562 source file (2024-02-27)
Supplement: Supplementary file 5 [file multiple_runs.tex]

\begin{table}[!ht]
    \centering
     \adjustbox{width=\linewidth}{\begin{tabular}{c|ccc|ccc|ccc}
    \hline
        \multirow{2}{*}{Runs} &  \multicolumn{3}{c|}{VoxelRCNN (5) } & \multicolumn{3}{c|}{VOTR-VoxelRCNN (3)} & \multicolumn{3}{c}{VOTR-TSD (5) } \\ 
         & Car  & Ped  & Cyc & Car  & Ped  & Cyc & Car  & Ped  & Cyc \\ 
        \hline
        Paper Run & 7.48 & 20.96 & 0.00 & 19.26 & 26.82 & 2.04 & 26.26 & 26.56 & 4.70  \\ 
        Mean & 8.22 & 20.26 & 0.00 & 20.17 & 27.63 & 1.43 & 27.1 & 26.42 & 4.4 \\ 
        %Std & 4.862235083 & 4.842626354 & 0 & 2.37394889 & 4.221733451 & 1.177794549 & 3.277906344 & 0.8153710812 & 2.183346056 \\ 
        \hline
    \end{tabular}}
    \caption{Results of Multiple Runs on the N$\rightarrow$K benchmark. We report the number of experiments between brackets.}
    \label{tab:multiple_runs}
    \vspace{-1em}
\end{table}
