# Supplementary material for: An Empirical Study of the Generalization Ability of Lidar 3D Object Detectors to Unseen Domains
Source: arXiv:2402.17562 source file (2024-02-27)
Supplement: Supplementary file 6 [file sensors_model.tex]

\begin{table*}[!ht]
    \centering
    \adjustbox{width=0.95\textwidth}{\begin{tabular}{c|cccc|cccc|cccc|c}
    \toprule
         \multirow{2}{*}{Method} & \multicolumn{4}{c|}{Car} & \multicolumn{4}{c|}{Ped} & \multicolumn{4}{c|}{Cyclist} & \multirow{2}{*}{mAP} \\ 
        
        ~ & Easy & Mod. & Hard & Mean & Easy & Mod. & Hard & Mean & Easy & Mod. & Hard & Mean & ~ \\
        \midrule
        \multicolumn{14}{c}{KITTI-64} \\
        \midrule
        PointRCNN & 89.64 & 80.55 & 78.03 & 82.74 & 64.93 & 57.64 & 49.84 & 57.47 & 91.25 & 71.35 & 66.77 & 76.46 & 72.22 \\ 
        PointPillars & 87.55 & 75.11 & 70.83 & 77.83 & 46.77 & 43.01 & 40.34 & 43.37 & 61.67 & 43.53 & 40.34 & 48.51 & 56.57 \\ 
        Second & 88.22 & 77.9 & 73.55 & 79.89 & 51 & 45.77 & 43.31 & 46.69 & 67.46 & 49.32 & 47.02 & 54.6 & 60.39 \\ 
        CenterPoint & 83.44 & 75.47 & 73.19 & 77.36 & 59.03 & 53.13 & 49.95 & 54.04 & 71.46 & 54.9 & 51.19 & 59.18 & 63.53 \\ 
        VoxelRCNN & 92.25 & 82.87 & 80.37 & 85.16 & 71.73 & 66.66 & 61.71 & 66.7 & 85.53 & 64.41 & 61.8 & 70.58 & 74.15 \\ 
        VOTR-VoxelRCNNhead & 92.18 & 82.48 & 79.9 & 84.85 & 66.52 & 61.84 & 56.98 & 61.78 & 75.42 & 58.95 & 56.15 & 63.51 & 70.05 \\ 
        PVRCNN & 91.26 & 82.51 & 80.22 & 84.66 & 64.51 & 58.45 & 55.4 & 59.45 & 83.51 & 62.49 & 59.86 & 68.62 & 70.91 \\ 
        PVRCNN Centerhead & 89.22 & 77.66 & 73.04 & 79.97 & 57.66 & 51.82 & 48.15 & 52.54 & 68.44 & 45.83 & 43.46 & 52.58 & 61.7 \\ 
        VOTR-TSD & 88.99 & 82.09 & 79.9 & 83.66 & 58.83 & 55 & 51.63 & 55.15 & 75.67 & 58.28 & 54.37 & 62.78 & 67.2 \\ 
       \midrule
       \multicolumn{14}{c}{KITTI-64 $\rightarrow$ KITTI-32} \\ 
       \midrule
        PointRCNN & 86.13 & 70.24 & 67.73 & 74.7 & 57.85 & 51.99 & 45.75 & 51.86 & 80.6 & 53.21 & 50.76 & 61.52 & 62.7 \\ 
        PointPillars & 81.8 & 67.22 & 62.42 & 70.48 & 39.11 & 35.3 & 33.01 & 35.81 & 35.47 & 21.63 & 20.69 & 25.93 & 44.07 \\ 
        Second & 85.21 & 69.94 & 65.35 & 73.5 & 45.22 & 40.96 & 37.15 & 41.11 & 50.68 & 34.17 & 32.44 & 39.1 & 51.24 \\ 
        CenterPoint & 81.06 & 67.93 & 64.55 & 71.18 & 46.65 & 42.49 & 38.99 & 42.71 & 58.77 & 38.03 & 35.76 & 44.19 & 52.69 \\ 
        VoxelRCNN & 87.9 & 73.63 & 69.33 & 76.96 & 61.53 & 56.71 & 51.88 & 56.71 & 66.37 & 43.25 & 40.91 & 50.18 & 61.28 \\ 
        VOTR-VoxelRCNNhead & 86.11 & 72.39 & 69.63 & 76.05 & 55.06 & 52.06 & 47.74 & 51.62 & 61.17 & 39.65 & 37.31 & 46.04 & 57.9 \\ 
        PVRCNN Centerhead & 85.78 & 67.48 & 60.91 & 71.39 & 49.51 & 44.19 & 40.21 & 44.64 & 48.03 & 28.34 & 26.24 & 34.2 & 50.08 \\ 
        PVRCNN & 88.05 & 74.42 & 70.4 & 77.62 & 59.39 & 54.1 & 48.38 & 53.96 & 64.94 & 44.95 & 41 & 50.3 & 60.63 \\ 
        VOTR-TSD & 86.15 & 72.66 & 70.07 & 76.29 & 54.26 & 49.34 & 45.73 & 49.78 & 64.29 & 43.62 & 41.38 & 49.76 & 58.61 \\ 
       \midrule
       \multicolumn{14}{c}{KITTI-64 $\rightarrow$ KITTI-16} \\ 
       \midrule 
        PointRCNN & 66.59 & 46.55 & 42.07 & 51.74 & 22.69 & 21.68 & 18.72 & 21.03 & 35.3 & 19.52 & 19.32 & 24.71 & 32.49 \\ 
        PointPillars & 67.64 & 48.5 & 43.35 & 53.16 & 23.06 & 20.35 & 18.08 & 20.5 & 12.47 & 7.76 & 7.6 & 9.28 & 27.65 \\ 
        Second & 65.76 & 45.63 & 40.74 & 50.71 & 18.56 & 16.61 & 14.81 & 16.63 & 24.46 & 14.3 & 13.99 & 17.58 & 28.3 \\ 
        CenterPoint & 67.13 & 48.03 & 43.24 & 52.8 & 16.37 & 15.15 & 13.82 & 15.11 & 20.33 & 11.58 & 10.9 & 14.27 & 27.39 \\ 
        VoxelRCNN & 69.63 & 51.54 & 47.17 & 56.11 & 30.23 & 27.43 & 24.06 & 27.24 & 34.69 & 20.2 & 19.03 & 24.64 & 36 \\ 
        VOTR-VoxelRCNNhead & 70.07 & 50.82 & 46.2 & 55.7 & 26.53 & 24.56 & 22.55 & 24.55 & 29.27 & 16.75 & 16.36 & 20.79 & 33.68 \\ 
        PVRCNN & 68 & 49.35 & 44.87 & 54.07 & 30.22 & 27.29 & 23.87 & 27.13 & 37.42 & 21.68 & 19.98 & 26.36 & 35.85 \\ 
        PVRCNN Centerhead & 59.51 & 39.7 & 33.51 & 44.24 & 18.38 & 15.53 & 12.26 & 15.39 & 17.1 & 10.49 & 8.48 & 12.02 & 23.88 \\ 
        VOTR-TSD & 69.28 & 50.97 & 46.59 & 55.61 & 23.92 & 21.55 & 19.66 & 21.71 & 34.62 & 19.33 & 19.19 & 24.38 & 33.9 \\ 
       \midrule
       \multicolumn{14}{c}{Oracle KITTI-32} \\
       \midrule 
        PointRCNN & 88.41 & 74.44 & 72.06 & 78.31 & 55.32 & 50.17 & 44.35 & 49.95 & 77.63 & 52.35 & 48.45 & 59.47 & 62.57 \\ 
        PointPillars & 83.3 & 69.36 & 65.2 & 72.62 & 47.26 & 41.8 & 38.61 & 42.56 & 51.68 & 32.9 & 31.24 & 38.6 & 51.26 \\ 
        Second & 86.85 & 72.91 & 70.07 & 76.61 & 46.94 & 41.08 & 36.28 & 41.43 & 65.3 & 43.14 & 40.77 & 49.74 & 55.93 \\ 
        CenterPoint & 80.65 & 69.87 & 68 & 72.84 & 53.54 & 48.69 & 45.45 & 49.23 & 63.35 & 44.04 & 41 & 49.46 & 57.18 \\ 
        VoxelRCNN & 89.52 & 77.07 & 74.3 & 80.3 & 60.41 & 53.1 & 47.94 & 53.82 & 78.6 & 54.33 & 51.43 & 61.46 & 65.19 \\ 
        PVRCNN & 91.86 & 77.5 & 74.99 & 81.45 & 59.38 & 50.72 & 45.16 & 51.75 & 77.2 & 55.7 & 51.77 & 61.55 & 64.92 \\ 
        VOTR-VoxelRCNNhead & 89 & 74.81 & 72.07 & 78.63 & 47.39 & 41.89 & 37.75 & 42.34 & 76.82 & 53.46 & 50.72 & 60.33 & 60.43 \\ 
        VOTR-TSD & 91.13 & 79.3 & 76.97 & 82.47 & 55.94 & 50.24 & 45.89 & 50.69 & 84.1 & 59.13 & 54.99 & 66.08 & 66.41 \\ 
       \midrule
       \multicolumn{14}{c}{Oracle KITTI-16} \\
       \midrule 
        PointRCNN & 81.2 & 61.05 & 56.8 & 66.35 & 51.31 & 45.25 & 39.75 & 45.44 & 66.86 & 39.72 & 37.6 & 48.06 & 53.28 \\ 
        PointPillars & 78.4 & 59.53 & 56.21 & 64.71 & 40.26 & 36.02 & 33.06 & 36.45 & 28.66 & 17.12 & 15.74 & 20.51 & 40.56 \\ 
        Second & 82.1 & 63.44 & 59.48 & 68.34 & 48.8 & 42.44 & 37.65 & 42.96 & 56.54 & 33.85 & 31.71 & 40.7 & 50.67 \\ 
        CenterPoint & 75.21 & 60.09 & 57.58 & 64.29 & 50.71 & 45.66 & 41.42 & 45.93 & 52.81 & 32.6 & 30.52 & 38.65 & 49.62 \\ 
        VoxelRCNN & 85.44 & 66.64 & 63.28 & 71.79 & 57.22 & 50.44 & 45.25 & 50.97 & 67.26 & 40.6 & 38.51 & 48.79 & 57.18 \\ 
        VOTR-VoxelRCNNhead & 82.82 & 63.86 & 59.03 & 68.57 & 47.67 & 40.92 & 35.66 & 41.42 & 57.37 & 35.4 & 33.36 & 42.04 & 50.68 \\ 
        PVRCNN  & 85.62 & 68.27 & 64.24 & 72.71 & 59.65 & 52.77 & 46.74 & 53.05 & 67.61 & 42.04 & 39.75 & 49.8 & 58.52 \\ 
        PVRCNN Centerhead & 82.29 & 65.85 & 61.5 & 69.88 & 56.71 & 51.72 & 46.02 & 51.48 & 54.18 & 31.77 & 29.59 & 38.51 & 53.29 \\ 
        VOTR-TSD & 85.77 & 69.22 & 66.27 & 73.75 & 60.07 & 52.58 & 47.69 & 53.45 & 68.35 & 43.05 & 40.67 & 50.69 & 59.3 \\ \hline
    \end{tabular}}
    \caption{Benchmarking different models on the KITTI dataset with different lines.}
    \label{tab:detailed_results_model_sensor}
\end{table*}
