# Supplementary material for: An Empirical Study of the Generalization Ability of Lidar 3D Object Detectors to Unseen Domains
Source: arXiv:2402.17562 source file (2024-02-27)
Supplement: Supplementary file 7 [file table_pvrcnn_votr_ros_3anchors.tex]

\begin{table}[t!]
    \centering
    \setlength{\tabcolsep}{1pt}
    \adjustbox{width=\linewidth}{\begin{tabular}{l|c|c|c}
        \toprule
        Model & Waymo  & W $\rightarrow$ K  & W $\rightarrow$ N \\ 
        \hline
        PVRCNN & 71.28 / 62.6  & 58.88 / 13.86  &  31.79 / 20.08 \\ 
        PVRCNN w/ ROS & 65.77 / 57.38 &  &  \\
        PVRCNN 3 Anchors &  &  &  \\
        PVRCNN 3 Anchors w/ ROS  &  &  &  \\ 
        \hline
        VOTR-TSD & 73.87 / 65.2 & 60.06	/ 14.47 & 35.83 / 21.66 \\ 
        VOTR-TSD w/ ROS &   &  &  \\
        VOTR-TSD 3 Anchors &  &  &  \\
        VOTR-TSD 3 Anchors w/ ROS  &  &  &  \\
        
        \bottomrule
    \end{tabular}}
    \caption{Investigating the OOD performance of anchor-based and anchorless detectors on Waymo $\rightarrow$ Kitti and Waymo $\rightarrow$ NuScenes.}
    \label{tab:anchorvslabel}
    \vspace{-1.8em}
\end{table}
