# Supplementary material for: An Empirical Study of the Generalization Ability of Lidar 3D Object Detectors to Unseen Domains
Source: arXiv:2402.17562 source file (2024-02-27)
Supplement: Supplementary file 8 [file table_pvrcnn_voxel_encoding.tex]

\begin{table*}[t!]
    \centering
    \adjustbox{width=0.95\textwidth}{\begin{tabular}{c|c|c|cccc|cccc|cccc}
    \hline
        \multirow{2}{*}{NPPV} & \multirow{2}{*}{Task} & \multirow{2}{*}{Class} & \multicolumn{4}{c|}{voxel height: 0.0625m} & \multicolumn{4}{c|}{voxel height: 0.1m} & \multicolumn{4}{c}{voxel height: 0.125m} \\
        ~ & ~ & ~ & Easy & Mod. & Hard & mAP & Easy & Mod. & Hard & mAP & Easy & Mod. & Hard & mAP \\ 
        \hline
        \multirow{9}{*}{4} & \multirow{3}{*}{64} & Car &  91.51  & 82.75  & 80.35  & 84.87  & 91.29  & 80.52  & 79.77  & 83.86  & 91.28  & 82.52  & 80.21  & 84.67  \\ 
        ~ & & Ped  ~ & 66.20  & 59.73  & 55.61  & 60.51  & 68.35  & 59.71  & 55.29  & 61.12  & 66.75  & 59.90  & 55.14  & 60.60  \\ 
        ~ & & Cyc  ~ & 84.22  & 62.81  & 60.11  & 69.05  & 81.42  & 62.41  & 59.72  & 67.85  & 84.90  & 64.03  & 60.08  & 69.67  \\ 
        \cline{2-15} 
        & \multirow{3}{*}{64 $\rightarrow$ 32} & Car ~ & 88.33  & 72.76  & 70.15  & 77.08  & 86.22  & 72.60  & 69.96  & 76.26  & 88.01  & 74.32  & 70.28  & 77.53  \\ 
        ~ & & Ped  ~ & 59.34  & 52.87  & 48.19  & 53.46  & 62.72  & 54.84  & 50.22  & 55.93  & 60.93  & 55.28  & 50.52  & 55.58  \\ 
        ~ & & Cyc  ~ & 65.28  & 41.83  & 39.73  & 48.94  & 65.67  & 42.27  & 40.21  & 49.38  & 70.56  & 45.91  & 43.68  & 53.38  \\ 
        \cline{2-15}
        & \multirow{3}{*}{64 $\rightarrow$ 16} & Car & 69.07  & 48.74  & 44.57  & 54.13  & 66.90  & 46.72  & 43.73  & 52.45  & 68.95  & 48.90  & 44.63  & 54.16  \\ 
        ~ & & Ped  ~ & 25.58  & 22.36  & 20.05  & 22.66  & 32.69  & 28.22  & 24.55  & 28.49  & 27.15  & 25.08  & 22.02  & 24.75  \\ 
        ~ & & Cyc  ~ & 34.02  & 19.61  & 18.01  & 23.88  & 36.04  & 22.04  & 20.08  & 26.06  & 39.24  & 22.61  & 20.61  & 27.49  \\ 
        \midrule
        \multirow{9}{*}{5} & \multirow{3}{*}{64} & Car &  91.66  & 82.73  & 80.30  & 84.90  & 91.26  & 82.51  & 80.22  & 84.66  & 91.61  & 82.72  & 80.38  & 84.90  \\ 
        ~ & & Ped  ~ & 68.06  & 61.28  & 57.04  & 62.13  & 64.51  & 58.45  & 55.40  & 59.45  & 67.66  & 60.47  & 57.40  & 61.84  \\ 
        ~ & & Cyc  ~ & 85.50  & 63.62  & 60.96  & 70.03  & 83.51  & 62.49  & 59.86  & 68.62  & 82.19  & 62.66  & 58.34  & 67.73  \\ 
        \cline{2-15}
        & \multirow{3}{*}{64 $\rightarrow$ 32} & Car ~ & 88.34  & 74.43  & 70.29  & 77.69  & 88.05  & 74.42  & 70.40  & 77.62  & 88.62  & 74.53  & 70.44  & 77.86  \\ 
        ~ & & Ped  ~ & 62.43  & 54.71  & 50.22  & 55.79  & 59.39  & 54.10  & 48.38  & 53.96  & 63.84  & 56.26  & 51.58  & 57.23  \\ 
        ~ & & Cyc  ~ & 66.46  & 43.49  & 41.52  & 50.49  & 64.94  & 44.95  & 41.00  & 50.30  & 67.15  & 44.03  & 41.78  & 50.99  \\ 
        \cline{2-15}
        & \multirow{3}{*}{64 $\rightarrow$ 16} & Car ~ & 68.65  & 48.72  & 44.43  & 53.93  & 68.00  & 49.35  & 44.87  & 54.07  & 71.18  & 49.52  & 45.07  & 55.26  \\ 
        ~ & & Ped  ~ & 24.40  & 22.46  & 19.27  & 22.04  & 30.22  & 27.29  & 23.87  & 27.13  & 37.90  & 33.49  & 29.44  & 33.61  \\ 
        ~ & & Cyc  ~ & 33.02  & 19.44  & 17.69  & 23.38  & 37.42  & 21.68  & 19.98  & 26.36  & 34.71  & 19.41  & 19.31  & 24.48  \\ 
        \midrule
        \multirow{9}{*}{7} & \multirow{3}{*}{64} & Car &  91.98  & 83.20  & 80.68  & 85.29  & 91.49  & 82.56  & 80.24  & 84.76  & 91.22  & 82.37  & 79.88  & 84.49  \\ 
        ~ & & Ped  ~ & 65.61  & 60.02  & 55.75  & 60.46  & 66.41  & 59.77  & 55.51  & 60.56  & 67.08  & 61.13  & 56.72  & 61.64  \\ 
        ~ & & Cyc  ~ & 82.59  & 61.25  & 57.15  & 67.00  & 85.26  & 63.93  & 59.74  & 69.64  & 84.35  & 63.02  & 60.45  & 69.28  \\ 
        \cline{2-15}
        & \multirow{3}{*}{64 $\rightarrow$ 32} & Car ~ & 88.92  & 73.29  & 70.39  & 77.53  & 86.66  & 73.01  & 70.26  & 76.64  & 86.48  & 72.85  & 70.18  & 76.50  \\ 
        ~ & & Ped  ~ & 64.72  & 57.28  & 50.97  & 57.66  & 63.00  & 56.40  & 51.60  & 57.00  & 59.72  & 53.52  & 48.89  & 54.05  \\ 
        ~ & & Cyc  ~ & 61.76  & 39.60  & 37.51  & 46.29  & 67.00  & 44.36  & 42.33  & 51.23  & 69.68  & 46.26  & 44.05  & 53.33  \\ 
        \cline{2-15}
        & \multirow{3}{*}{64 $\rightarrow$ 16} & Car ~ & 68.50  & 47.60  & 42.90  & 53.00  & 67.47  & 47.39  & 42.90  & 52.59  & 67.46  & 48.63  & 44.21  & 53.43  \\ 
        ~ & & Ped  ~ & 33.31  & 28.28  & 25.82  & 29.14  & 33.21  & 28.42  & 26.21  & 29.28  & 28.19  & 25.97  & 22.76  & 25.64  \\ 
        ~ & & Cyc  ~ & 36.29  & 20.37  & 20.11  & 25.59  & 29.15  & 17.40  & 15.50  & 20.68  & 32.81  & 19.16  & 17.54  & 23.17  \\ 
        \midrule
        \multirow{9}{*}{9} & \multirow{3}{*}{64} & Car &  90.94  & 82.27  & 79.98  & 84.40  & 91.48  & 82.45  & 80.08  & 84.67  & 91.45  & 82.55  & 80.18  & 84.73  \\ 
        ~ & & Ped  ~ & 65.81  & 59.39  & 55.18  & 60.12  & 66.31  & 60.82  & 56.43  & 61.19  & 65.06  & 59.11  & 55.08  & 59.75  \\ 
        ~ & & Cyc  ~ & 81.89  & 60.03  & 57.68  & 66.53  & 85.92  & 64.95  & 62.11  & 70.99  & 85.81  & 62.03  & 57.69  & 68.51  \\ 
        \cline{2-15}
        & \multirow{3}{*}{64 $\rightarrow$ 32} & Car ~ & 88.13  & 72.47  & 69.85  & 76.82  & 88.61  & 73.03  & 70.38  & 77.34  & 88.90  & 74.68  & 70.41  & 77.99  \\ 
        ~ & & Ped  ~ & 62.47  & 55.82  & 49.69  & 55.99  & 64.51  & 57.59  & 51.63  & 57.91  & 61.33  & 55.63  & 50.86  & 55.94  \\ 
        ~ & & Cyc  ~ & 67.95  & 44.07  & 41.97  & 51.33  & 70.05  & 44.51  & 42.30  & 52.29  & 72.27  & 47.75  & 43.66  & 54.56  \\ 
        \cline{2-15}
        & \multirow{3}{*}{64 $\rightarrow$ 16} & Car ~ & 68.27  & 46.90  & 42.56  & 52.57  & 68.99  & 49.08  & 44.46  & 54.18  & 69.82  & 49.49  & 45.02  & 54.77  \\ 
        ~ & & Ped  ~ & 26.31  & 22.62  & 19.37  & 22.77  & 34.88  & 30.80  & 27.32  & 31.00  & 30.77  & 27.13  & 23.82  & 27.24  \\ 
        ~ & & Cyc  ~ & 31.56  & 18.04  & 17.65  & 22.42  & 34.52  & 20.80  & 19.42  & 24.91  & 38.28  & 22.21  & 20.40  & 26.96 \\ \hline
    \end{tabular}}
    \caption{PVRCNN-Voxel Encoding}
    \label{tab:pvrcnn_voxel_encoding}
\end{table*}
