# Supplementary material for: An Empirical Study of the Generalization Ability of Lidar 3D Object Detectors to Unseen Domains
Source: arXiv:2402.17562 source file (2024-02-27)
Supplement: Supplementary file 9 [file table_second_voxel_encoding.tex]

\begin{table*}[!ht]
    \centering
    \adjustbox{width=0.95\textwidth}{\begin{tabular}{c|c|c|cccc|cccc|cccc}
    \hline
       \multirow{2}{*}{NPPV} & \multirow{2}{*}{Task} & \multirow{2}{*}{Class} & \multicolumn{4}{c|}{voxel height: 0.0625m} & \multicolumn{4}{c|}{voxel height: 0.1m} & \multicolumn{4}{c}{voxel height: 0.125m} \\
        ~ & ~ & ~ & Easy & Mod. & Hard & mAP & Easy & Mod. & Hard & mAP & Easy & Mod. & Hard & mAP \\ 
        \hline 
        \multirow{9}{*}{4} & \multirow{3}{*}{64} & Car/3D & 87.63  & 78.00  & 75.32  & 80.31  & 89.70  & 78.47  & 75.26  & 81.14  & 88.33  & 76.38  & 73.63  & 79.45  \\ 
        ~ & ~ & Ped./3d & 49.82  & 44.80  & 41.45  & 45.36  & 52.75  & 47.70  & 44.03  & 48.16  & 50.10  & 45.34  & 41.74  & 45.73  \\ 
        ~ & ~ & Cyc./3D & 66.89  & 49.20  & 46.85  & 54.31  & 66.92  & 51.51  & 47.65  & 55.36  & 69.13  & 49.82  & 46.20  & 55.05  \\
        \cline{2-15}
        ~ & \multirow{3}{*}{64$\rightarrow$32} & Car/3D & 84.38  & 68.36  & 65.19  & 72.64  & 84.57  & 68.35  & 65.03  & 72.65  & 84.10  & 68.15  & 64.53  & 72.26  \\
        ~ & ~ & Ped./3d & 44.43  & 40.36  & 36.62  & 40.47  & 45.43  & 39.89  & 36.04  & 40.46  & 46.27  & 42.61  & 38.83  & 42.57  \\ 
        ~ & ~ & Cyc./3D & 48.55  & 31.65  & 29.68  & 36.62  & 52.38  & 36.06  & 33.87  & 40.77  & 54.93  & 36.95  & 34.15  & 42.01  \\ 
        \cline{2-15}
        ~ & \multirow{3}{*}{64$\rightarrow$16} & Car/3D & 61.88  & 43.41  & 38.92  & 48.07  & 63.02  & 44.90  & 40.48  & 49.47  & 65.01  & 45.53  & 39.89  & 50.15  \\
        ~ & ~ & Ped./3d & 21.39  & 18.86  & 15.91  & 18.72  & 20.06  & 17.21  & 15.47  & 17.58  & 21.32  & 20.00  & 17.19  & 19.50  \\ 
        ~ & ~ & Cyc./3D & 23.89  & 13.56  & 13.34  & 16.93  & 25.72  & 14.40  & 14.12  & 18.08  & 31.34  & 18.28  & 16.94  & 22.18  \\ 
        \midrule
        \multirow{9}{*}{5} & \multirow{3}{*}{64} & Car/3D & 88.20  & 78.14  & 75.16  & 80.50  & 88.22  & 77.90  & 73.55  & 79.89  & 88.04  & 76.98  & 73.09  & 79.37  \\ 
        ~ & ~ & Ped./3d & 52.27  & 48.06  & 44.56  & 48.30  & 51.00  & 45.77  & 43.31  & 46.69  & 47.30  & 44.01  & 41.02  & 44.11  \\ 
        ~ & ~ & Cyc./3D & 63.09  & 48.39  & 45.81  & 52.43  & 67.46  & 49.32  & 47.02  & 54.60  & 64.62  & 49.69  & 47.04  & 53.78  \\ 
        \cline{2-15}
        ~ & \multirow{3}{*}{64$\rightarrow$32} & Car/3D & 83.38  & 67.55  & 64.21  & 71.71  & 85.21  & 69.94  & 65.35  & 73.50  & 84.10  & 67.92  & 64.56  & 72.19  \\
        ~ & ~ & Ped./3d & 46.01  & 41.95  & 38.39  & 42.11  & 45.22  & 40.96  & 37.15  & 41.11  & 38.25  & 36.26  & 34.17  & 36.23  \\ 
        ~ & ~ & Cyc./3D & 50.72  & 33.39  & 31.66  & 38.59  & 50.68  & 34.17  & 32.44  & 39.10  & 51.93  & 35.11  & 31.98  & 39.68  \\ 
        \cline{2-15}
        ~ & \multirow{3}{*}{64$\rightarrow$16} & Car/3D & 63.26  & 43.92  & 39.24  & 48.81  & 65.76  & 45.63  & 40.74  & 50.71  & 65.26  & 46.14  & 41.23  & 50.88  \\
        ~ & ~ & Ped./3d & 23.15  & 20.47  & 18.54  & 20.72  & 18.56  & 16.51  & 14.81  & 16.63  & 19.86  & 18.87  & 16.52  & 18.41  \\ 
        ~ & ~ & Cyc./3D & 21.70  & 12.58  & 12.37  & 15.55  & 24.46  & 14.30  & 13.99  & 17.58  & 24.24  & 13.22  & 12.78  & 16.75  \\ 
        \midrule
        \multirow{9}{*}{7} & \multirow{3}{*}{64} & Car/3D & 88.16  & 78.52  & 75.73  & 80.80  & 88.26  & 76.07  & 73.45  & 79.26  & 88.38  & 77.82  & 73.68  & 79.96  \\ 
        ~ & ~ & Ped./3d & 53.85  & 48.85  & 45.03  & 49.24  & 54.24  & 49.34  & 45.34  & 49.64  & 49.92  & 45.86  & 42.20  & 45.99  \\ 
        ~ & ~ & Cyc./3D & 69.19  & 53.68  & 49.83  & 57.56  & 69.77  & 50.58  & 47.96  & 56.11  & 70.74  & 51.23  & 47.59  & 56.52  \\ 
        \cline{2-15}
        ~ & \multirow{3}{*}{64$\rightarrow$32} & Car/3D & 84.50  & 68.39  & 65.15  & 72.68  & 84.46  & 68.11  & 63.38  & 71.98  & 84.51  & 68.17  & 64.70  & 72.46  \\
        ~ & ~ & Ped./3d & 46.67  & 41.38  & 37.38  & 41.81  & 47.95  & 42.33  & 38.26  & 42.85  & 46.64  & 42.33  & 38.64  & 42.54  \\ 
        ~ & ~ & Cyc./3D & 56.17  & 37.31  & 34.93  & 42.80  & 52.97  & 35.77  & 33.67  & 40.80  & 55.40  & 35.26  & 33.05  & 41.24  \\ 
        \cline{2-15}
        ~ & \multirow{3}{*}{64$\rightarrow$16} & Car/3D & 61.73  & 43.34  & 38.85  & 47.97  & 64.30  & 44.94  & 39.47  & 49.57  & 64.67  & 45.68  & 40.79  & 50.38  \\
        ~ & ~ & Ped./3d & 19.40  & 17.58  & 14.96  & 17.31  & 19.35  & 17.82  & 15.30  & 17.49  & 19.57  & 18.61  & 16.03  & 18.07  \\ 
        ~ & ~ & Cyc./3D & 26.86  & 15.16  & 13.57  & 18.53  & 27.37  & 15.99  & 14.73  & 19.36  & 26.26  & 14.90  & 14.75  & 18.64  \\
        \midrule
        \multirow{9}{*}{9} & \multirow{3}{*}{64} & Car/3D & 86.47  & 74.95  & 72.47  & 77.96  & 88.40  & 77.85  & 73.43  & 79.89  & 87.55  & 75.74  & 73.13  & 78.80  \\ 
        ~ & ~ & Ped./3d & 55.72  & 50.13  & 45.92  & 50.59  & 52.73  & 47.74  & 44.32  & 48.26  & 55.09  & 49.26  & 45.41  & 49.92  \\ 
        ~ & ~ & Cyc./3D & 68.48  & 53.09  & 49.13  & 56.90  & 70.03  & 51.47  & 47.62  & 56.37  & 66.32  & 49.50  & 46.79  & 54.21  \\
        \cline{2-15}
        ~ & \multirow{3}{*}{64$\rightarrow$32} & Car/3D & 81.04  & 65.00  & 62.06  & 69.37  & 84.65  & 67.89  & 64.47  & 72.34  & 83.34  & 67.50  & 62.96  & 71.27  \\
        ~ & ~ & Ped./3d & 49.50  & 43.23  & 39.19  & 43.97  & 47.03  & 42.50  & 38.14  & 42.56  & 46.83  & 42.69  & 38.76  & 42.76  \\ 
        ~ & ~ & Cyc./3D & 51.60  & 34.10  & 32.14  & 39.28  & 52.15  & 34.60  & 32.68  & 39.81  & 50.10  & 34.77  & 32.12  & 39.00  \\
        \cline{2-15}
        ~ & \multirow{3}{*}{64$\rightarrow$16} & Car/3D & 58.60  & 40.70  & 36.50  & 45.27  & 64.38  & 44.07  & 39.33  & 49.26  & 65.18  & 44.47  & 39.56  & 49.74  \\ 
        ~ & ~ & Ped./3d & 20.68  & 17.97  & 14.83  & 17.83  & 17.63  & 15.45  & 13.71  & 15.60  & 20.52  & 18.61  & 16.76  & 18.63  \\ 
        ~ & ~ & Cyc./3D & 21.00  & 11.91  & 11.96  & 14.96  & 24.87  & 14.78  & 13.94  & 17.86  & 25.53  & 14.84  & 13.60  & 17.99 \\ \hline
    \end{tabular}}
    \caption{Second: Voxel Encoding}
    \label{tab:second_voxel_encoding}
\end{table*}
