# Supplementary material for: An Empirical Study of the Generalization Ability of Lidar 3D Object Detectors to Unseen Domains
Source: arXiv:2402.17562 source file (2024-02-27)
Supplement: Supplementary file 10 [file table_votr_voxel_encoding.tex]

\begin{table*}[t!]
    \centering
    \adjustbox{width=0.90\textwidth}{\begin{tabular}{c|c|c|cccc|cccc|cccc}
    \hline
        \multirow{2}{*}{NPPV} & \multirow{2}{*}{Task} & \multirow{2}{*}{Class} &  \multicolumn{4}{c|}{voxel height: $0.0625m$} & \multicolumn{4}{c|}{voxel height: $0.1m$} & \multicolumn{4}{c}{voxel height: $0.125m$} \\ 
        ~ &~ &~ & Easy & Mod. & Hard & mAP & Easy & Mod. & Hard & mAP & Easy & Mod. & Hard & mAP \\ 
        \midrule
        \multirow{9}{*}{4} & \multirow{3}{*}{64} & Car & 91.50  & 82.93  & 80.35  & 84.93  & 89.08  & 80.28  & 77.81  & 82.39  & 88.96  & 79.62  & 77.11  & 81.90  \\ 
        & ~ & Ped. & 59.09  & 55.87  & 51.31  & 55.42  & 53.98  & 50.30  & 47.29  & 50.52  & 62.75  & 57.15  & 53.17  & 57.69  \\ 
        & ~ & Cyc. & 75.29  & 55.41  & 53.00  & 61.23  & 79.77  & 60.05  & 56.02  & 65.28  & 74.82  & 56.68  & 54.06  & 61.85  \\ 
        \cline{2-15}
        & \multirow{3}{*}{64 $\rightarrow 32$} & Car &  86.67  & 74.85  & 72.18  & 77.90  & 85.88  & 72.24  & 69.58  & 75.90  & 86.24  & 72.18  & 69.42  & 75.95  \\ 
        &~ & Ped. &  56.01  & 51.08  & 46.97  & 51.36  & 50.33  & 46.72  & 43.26  & 46.77  & 62.09  & 56.40  & 50.78  & 56.42  \\ 
       & ~ & Cyc. &  65.91  & 43.37  & 41.15  & 50.15  & 61.79  & 42.72  & 40.40  & 48.31  & 68.12  & 45.55  & 43.27  & 52.31  \\ 
        \cline{2-15}
        & \multirow{3}{*}{64 $\rightarrow$ 16} & Car &  71.64  & 53.14  & 48.75  & 57.84  & 68.83  & 50.45  & 45.97  & 55.08  & 72.03  & 51.54  & 47.08  & 56.88  \\ 
        &~ & Ped. &  27.76  & 24.85  & 22.97  & 25.19  & 29.17  & 25.50  & 23.64  & 26.10  & 41.22  & 36.71  & 32.98  & 36.97  \\ 
       & ~ & Cyc. &  31.66  & 18.99  & 17.22  & 22.62  & 33.48  & 20.15  & 18.53  & 24.06  & 41.68  & 23.11  & 22.93  & 29.24  \\ 
        \midrule
        \multirow{9}{*}{5} & \multirow{3}{*}{64} & Car &  91.12  & 82.24  & 79.98  & 84.45  & 88.99  & 82.09  & 79.90  & 83.66  & 89.45  & 82.33  & 80.11  & 83.96  \\ 
        &~ & Ped. &  55.91  & 53.31  & 49.64  & 52.95  & 58.83  & 55.00  & 51.63  & 55.15  & 60.59  & 56.57  & 53.26  & 56.81  \\ 
       & ~ & Cyc. &  70.13  & 54.09  & 51.50  & 58.57  & 75.67  & 58.28  & 54.37  & 62.78  & 75.17  & 56.87  & 54.27  & 62.11  \\ 
        \cline{2-15}
        & \multirow{3}{*}{64 $\rightarrow$ 32} & Car &  86.21  & 74.68  & 72.12  & 77.67  & 86.15  & 72.66  & 70.07  & 76.29  & 86.42  & 74.64  & 72.18  & 77.75  \\ 
        &~ & Ped. &  51.19  & 47.66  & 44.29  & 47.72  & 54.26  & 49.34  & 45.73  & 49.78  & 57.15  & 52.61  & 48.72  & 52.83  \\ 
       & ~ & Cyc. &  57.81  & 39.35  & 37.08  & 44.75  & 64.29  & 43.62  & 41.38  & 49.76  & 65.04  & 45.50  & 43.30  & 51.28  \\ 
        \cline{2-15}
        & \multirow{3}{*}{64 $\rightarrow$ 16} & Car &  71.64  & 53.18  & 48.80  & 57.87  & 69.28  & 50.97  & 46.59  & 55.61  & 71.73  & 53.28  & 48.97  & 57.99  \\ 
        &~ & Ped. &  27.23  & 23.26  & 20.25  & 23.58  & 23.92  & 21.55  & 19.66  & 21.71  & 32.53  & 30.22  & 26.81  & 29.85  \\ 
       & ~ & Cyc. &  29.64  & 17.72  & 17.62  & 21.66  & 34.62  & 19.33  & 19.19  & 24.38  & 37.77  & 21.13  & 20.80  & 26.57  \\ 
        \midrule
        \multirow{9}{*}{7} & \multirow{3}{*}{64} & Car & 88.20  & 79.57  & 77.18  & 81.65  & 91.48  & 82.77  & 80.34  & 84.86  & 88.38  & 79.61  & 76.94  & 81.64  \\ 
         &~ & Ped. &  50.21  & 47.77  & 44.09  & 47.35  & 57.19  & 55.30  & 52.60  & 55.03  & 57.41  & 53.41  & 50.21  & 53.67  \\ 
       & ~ & Cyc. &  73.45  & 55.91  & 53.37  & 60.91  & 72.43  & 56.46  & 52.69  & 60.53  & 64.51  & 50.41  & 48.21  & 54.38  \\ 
        \cline{2-15}
        & \multirow{3}{*}{64 $\rightarrow$ 32} & Car &  85.13  & 71.74  & 69.11  & 75.32  & 88.25  & 74.93  & 72.34  & 78.51  & 85.39  & 71.67  & 68.93  & 75.33  \\ 
         &~ & Ped. &  49.36  & 45.42  & 42.13  & 45.64  & 55.51  & 51.36  & 47.69  & 51.52  & 59.26  & 54.31  & 49.35  & 54.31  \\ 
       & ~ & Cyc. &  62.05  & 43.22  & 41.12  & 48.80  & 62.94  & 43.78  & 40.29  & 49.00  & 60.85  & 42.01  & 41.47  & 48.11  \\ 
        \cline{2-15}
        & \multirow{3}{*}{64 $\rightarrow$ 16} & Car &  69.79  & 50.53  & 47.71  & 56.01  & 70.32  & 51.39  & 48.42  & 56.71  & 69.80  & 52.14  & 47.93  & 56.62  \\ 
         &~ & Ped. &  29.78  & 27.05  & 23.76  & 26.86  & 30.27  & 27.82  & 25.60  & 27.90  & 31.97  & 28.99  & 25.60  & 28.85  \\ 
       & ~ & Cyc. &  37.55  & 22.29  & 20.77  & 26.87  & 34.41  & 19.98  & 18.57  & 24.32  & 39.69  & 22.73  & 22.41  & 28.28  \\ 
        \midrule
         \multirow{9}{*}{9} & \multirow{3}{*}{64} & Car &88.81  & 80.03  & 77.46  & 82.10  & 88.84  & 80.33  & 77.57  & 82.25  & 89.40  & 80.31  & 77.80  & 82.50  \\ 
         &~ & Ped. &  55.46  & 52.45  & 48.12  & 52.01  & 49.33  & 46.05  & 43.83  & 46.40  & 52.97  & 50.75  & 48.27  & 50.66  \\ 
       & ~ & Cyc. &  75.44  & 56.87  & 52.98  & 61.76  & 76.33  & 55.53  & 52.94  & 61.60  & 72.30  & 54.31  & 51.74  & 59.45  \\ 
        \cline{2-15}
        & \multirow{3}{*}{64 $\rightarrow$ 32} & Car &  85.96  & 71.90  & 69.23  & 75.70  & 86.00  & 72.15  & 69.30  & 75.82  & 86.38  & 72.59  & 69.88  & 76.28  \\ 
         &~ & Ped. &  51.32  & 47.20  & 43.65  & 47.39  & 45.25  & 42.32  & 40.62  & 42.73  & 56.36  & 51.50  & 47.69  & 51.85  \\ 
       & ~ & Cyc. &  66.44  & 44.74  & 40.94  & 50.71  & 63.45  & 45.44  & 41.76  & 50.22  & 63.42  & 44.47  & 42.37  & 50.09  \\ 
        \cline{2-15}
        & \multirow{3}{*}{64 $\rightarrow$ 16} & Car &  68.95  & 50.74  & 47.82  & 55.84  & 70.09  & 50.82  & 46.35  & 55.75  & 69.28  & 50.69  & 46.27  & 55.42  \\ 
         &~ & Ped. &  26.68  & 23.92  & 20.98  & 23.86  & 20.41  & 19.52  & 18.09  & 19.34  & 29.50  & 25.90  & 24.14  & 26.51  \\ 
       & ~ & Cyc. &  38.16  & 22.77  & 20.97  & 27.30  & 37.13  & 21.55  & 19.69  & 26.12  & 44.46  & 25.49  & 25.43  & 31.79 \\ \hline
    \end{tabular}}
    \caption{ VOTR-TSD: Voxel Encoding}
    \label{tab:votr_voxel_encoding}
\end{table*}
